# Supplementary material for: Deep Analysis of CNN-based Spatio-temporal Representations for Action Recognition
Source: arXiv:2010.11757 source file (2021-03-29)
Supplement: Supplementary file 6 [file temporal_analysis.tex]

\begin{table}[t]
    \centering
    \begin{adjustbox}{max width=\linewidth}
    \begin{tabular}{c|c|c|c|c}
        \toprule
             & \multicolumn{2}{c|}{SSV2} & \multicolumn{2}{c}{Kinetics}  \\
        \cmidrule{2-5}
                     & Temporal       &  Static    & Temporal & Static \\
        \midrule
        Class overlap ratio & 38.89\% &  11.11\% & 21.88\% & 3.12\% \\
        \midrule
        Human~\cite{temporal_dataset}   & 79.7\% (+47.8\%) & 71.1 (+31.7\%) & 75.0\% (+8.4\%) & 76.4\% (+8.2\%) \\
        Machine (Ours)    & 80.6\% (+68.9\%) & 83.4 (+24.7\%) & 73.5\% (+22.1\%) & 92.7\% (-1.7\%) \\
        \bottomrule
        % \multicolumn{8}{l}{\footnotesize{There is a performance of I3D and S3D from the original paper is b}}
    \end{tabular}
    \end{adjustbox}
    % \vspace{-2mm}
    \caption{The class overlap ratio, recognition accuracies and average temporal gains (in parenthesis) of the temporal and static datasets identified by human and machine.}
    \label{table:temporal_analysis}
    
\end{table}
