# Supplementary material for: Deep Analysis of CNN-based Spatio-temporal Representations for Action Recognition
Source: arXiv:2010.11757 source file (2021-03-29)
Supplement: Supplementary file 7 [file temporal_dynamics.tex]

\mycomment {
\begin{table}[t]
    \caption{Temporal dynamic analysis by removing machine-identified temporal classes on \Kinetics.}
    \label{table:temporal_dynamics}
    \centering
    \begin{adjustbox}{max width=\linewidth}
    \begin{tabular}{c|c|c|c|c|c}
        \toprule
             & \# of classes & TAM Acc. & ATG-all & ATG-tc & ATG-tc2 \\
        \midrule
        Original & 400 & 74.24\% & 5.07\% & 16.93\% & 7.00\% \\
        Round 1 & 360 & 74.91\% & 4.16\%  & 13.84\% & 5.94\% \\
        Round 2 & 320 & 76.39\% & 3.79\%  & 12.68\% & 12.68\% \\        % 72.6020
        \bottomrule
    \end{tabular}
    \end{adjustbox}
\end{table}
}

\begin{table}[t]
    \centering
    \begin{adjustbox}{max width=.85\linewidth}
    \begin{tabular}{c|c|c|c|c}
        \toprule
             & \# of classes & TAM Acc. & ATG-all & ATG-tc \\
        \midrule
        Original & 400 & 74.24\% & 5.07\% & 16.93\%  \\
        Round 1 & 360 & 74.91\% & 4.16\%  & 13.84\%  \\
        Round 2 & 320 & 76.39\% & 3.79\%  & 12.68\%  \\        % 72.6020
        \bottomrule
    \end{tabular}
    \end{adjustbox}
    % \vspace{-2mm}
    \caption{Results of temporality analysis on \Kinetics by removing temporal classes.}
    \label{table:temporal_dynamics}
\end{table}
